# Supplementary material for: Stein Variational Adaptive Importance Sampling
Source: arXiv:1704.05201 source file (2017-07-25)
Supplement: Supplementary file 1 [file appendix.tex]

\section*{Theoretical Investigation of SteinIS}
\subsection{Proof of Theorem 1}
Let $\widetilde{\mu}^j_N(d\bd{x})$ be the empirical measure of $\{\bd{z}^j_i\}_{i=1}^N$ and $\hat{\mu}^j_M(d\bd{x})$ be the empirical measure of $\{\bd{y}^j_i\}_{i=1}^M.$ We use $\mu_{\infty}^j$ the exact probability measure of $\bd{z}^j$ defined in equation \eqref{transform} and \eqref{stein}. We define the Lipschitz metric between two probability measures  as
\begin{equation*}
\mathrm{BL}(\mu, \nu)=\sup_f{\mathbb{E}_\mu f-\mathbb{E}_\nu f, \quad \textit{s.t.}\quad \|f\|_{\mathrm{BL}}\le 1},
\end{equation*}
\begin{equation*}
\textit{where } \|f\|_{\mathrm{BL}}= \max\{\sup_{\bd{x}}f(\bd{x}), \sup_{\bd{x}\neq \bd{y}} \frac{|f(\bd{x})-f(\bd{y})|}{\|\bd{x}-\bd{y}\|_2}\}.
\end{equation*}

\begin{thm}
Suppose $\{\bd{z}^0_i\}_{i=1}^N$ and $\{\bd{y}^0_i\}_{i=1}^M$ are drawn from the distribution with probability measure $\mu_{\infty}^0.$ Assume
\begin{equation*}
\lim_{N\rightarrow\infty}\mathrm{BL}(\widetilde{\mu}^0_N, \mu_{\infty}^0)=0, \quad \lim_{M\rightarrow\infty}\mathrm{BL}(\hat{\mu}^0_M, \mu_{\infty}^0)=0,
\end{equation*}
then for $j=1,2,\cdots, K$, we have
$$\lim_{N\rightarrow\infty}\mathrm{BL}(\hat{\mu}^j_N, \mu_{\infty}^j)=0. $$
\end{thm}

{\bf Proof:} Based on the following inequality
\begin{equation*}
%\begin{split}
\|\bd{T}_{\mu, p}\mu - \bd{T}_{\widetilde{\mu}, p}\hat{\mu}\|_{\mathrm{BL}}\le \|\bd{T}_{\mu, p}\mu - \bd{T}_{\widetilde{\mu}, p}\widetilde{\mu}\|_{\mathrm{BL}}+\|\bd{T}_{\widetilde{\mu}, p}\widetilde{\mu} - \bd{T}_{\widetilde{\mu}, p}\hat{\mu}\|_{\mathrm{BL}},
%\end{split}
\end{equation*}
Since we know $\mathrm{BL}(\widetilde{\mu}^0_N, \hat{\mu}^0_M)\rightarrow 0,$ then it is easy to derive $\mathrm{BL}(\hat{\mu}^1_M, \mu_{\infty}^1)\rightarrow 0.$
Similarly, $\mathrm{BL}(\hat{\mu}^j_N, \mu_{\infty}^j)\rightarrow 0$ can be proved inductively.

\subsection{Proof of Theorem 3}
{\bf Proof:} Denote $A(X^t,t)=\int_\Omega q(x,t)[\nabla_x \log p(x)K(x,X^t)+\nabla_x K(x,X^t)]dx,$ to prove equation (\ref{diffode}), we just need to show for any test function $\psi(x,t)\in C^{2,1}_0$ ($C^{2,1}_0$ means the set of functions which are second-order differential in $x$ and first-order differential in $t$ and take zeros when $x\in \partial\Omega$), we have
\begin{equation}
\int (\frac{\partial \rho(x,t)}{\partial t}+\mathrm{div}(\rho(x,t)A(x,t)))\psi(x,t)dx=0.
\end{equation}
Let $\mathfrak{F}_t=\sigma(X^s: s\le t),$ and define un-normalized conditional probability $p_{(t)}(\psi_t)=\mathrm{E}[\psi(X^t,t)\mid \mathfrak{F}_t].$
By Ito's formula,
\begin{equation}
\label{ito}
d\psi(X^t,t)=\nabla_x\psi\cdot dX^t+\frac{\partial \psi}{\partial t}dt=[-\nabla_x\psi\cdot A(X^t,t)+\frac{\partial \psi}{\partial t}]dt.
\end{equation}
As $\rho(x,t)$ is the probability density function of $X^t$, by the definition of conditional probability, it satisfies
 \begin{equation}
 \label{formu}
p_{(t)}(\psi_t)=\int \rho(x,t)\psi(x,t)dx.
 \end{equation}

According to the formula (\ref{ito}), we have the following identity,
\begin{equation}
\label{inte}
\psi(X^t,t)=\psi(X^0,0)+\int_0^t[-\nabla_x\psi\cdot A(X^s,s)+\frac{\partial \psi}{\partial t}]ds.
\end{equation}
Based on (\ref{inte}), we have
\begin{equation}
\label{equa}
\mathrm{E}[\psi(X^t,t)\mid \mathfrak{F}_t]=\mathrm{E}[\psi(X^0,0)\mid \mathfrak{F}_t]+\mathrm{E}[\int_0^t(-\nabla_x\psi\cdot A(X^s,s)+\frac{\partial \psi}{\partial t})ds\mid \mathfrak{F}_t].
\end{equation}
By the definition of condition probability and Fubini's theorem, and based on the equality (\ref{formu}), (\ref{equa}), we have
\begin{equation}
\label{fina}
\int \rho(x,t)\psi(x,t)dx=\int \rho(x,0)\psi(x,0)dx+\int \int_0^t\rho(x,s)[-\nabla_x\psi\cdot A(x,s)+\frac{\partial \psi}{\partial t}]dsdx.
\end{equation}
We observe the following formula, $$\nabla_x\psi\cdot (\rho(x,s)A(x,s))=\nabla_x\cdot(\psi A(x,s)\rho(x,s))-\psi\nabla_x\cdot (\rho(x,s)A(x,s)).$$ Since $\psi(x,s)\in C^{2,1}_0$, then we have $\int_\Omega \nabla_x\cdot(\psi\rho(x,s) A(X^s,s))dx=0$ for any $s$. It is easy to verify that
\begin{equation*}
\begin{split}
\int_\Omega\int_0^t \frac{\partial(\rho\psi)}{\partial t}dsdx &=\int_\Omega\int_0^t (\psi\frac{\partial\rho}{\partial t}+\rho\frac{\partial\psi}{\partial t})dsdx \\
&=\int_\Omega \rho(x,t)\psi(x,t)dx-\int_\Omega \rho(x,0)\psi(x,0)dx.
\end{split}
\end{equation*}
Equation (\ref{fina}) can be rewritten in the following,
\begin{equation}
\int_0^t\int_\Omega [\frac{\partial \rho }{\partial t}+\nabla\cdot(\rho(x,s)A(x,s))]\psi(x,s)dxds=0.
\end{equation}
Take derivative w.r.t. $t$, we have
\begin{equation}
\label{final}
\int_\Omega [\frac{\partial \rho }{\partial t}+\nabla\cdot(\rho(x,t)A(x,t))]\psi(x,s) dx=0.
\end{equation}
Since equation (\ref{final}) holds for any test function $\psi(x,t)\in C^{2,1}_0$, then we can get $\frac{\partial \rho }{\partial t}=-\nabla\cdot(\rho(x,t)A(x,t)).$ The proof is complete. $\square$
